# Supplementary material for: Anomaly Inflow, Accidental Symmetry, and Spontaneous Symmetry Breaking
Source: arXiv:1910.07549 source file (2019-10-16)
Supplement: Supplementary file 1 [file sec_appendix.tex]

%!TEX root = ./GMSWmain.tex

\section{Einstein metric on $M_4$}

We consider the following ansatz for the metric on $M_4$,
\begin{align}  
ds^2(M_4) = h_1 \, d\mu^2 + \frac{1}{4}  \, h_2 \, D \widetilde{\psi}^2 + \frac{1}{4} (1-\mu^2) ds^2(S^2_\varphi), \qquad D  \widetilde{\psi} &= d  \psi +v \,  \cos \theta \,  d\varphi ,
\end{align}
where $h_1$, $h_2$ are function of $\mu$ and $v$ is a constant.
%Since $h_2$ is arbitrary, we can impose without loss of generality
%that the period of $\psi$ is $2\pi$.  
The coordinate $\widetilde{\psi}$ parametrizes a circle whose period will be fixed by regularity conditions below.
This metric 
satisfies the Einstein condition
$R_{mn} = K \, g_{mn}$ provided
that
\begin{align}
h_1' & = 
\frac{h_1 \left(h_1 \left(3 h_2 v^2+\left(\mu ^2-1\right) \left(K \left(\mu
   ^2-1\right)+4\right)\right)+\mu ^2-2\right)}{\mu  \left(\mu ^2-1\right)} \ ,  \label{eqno1}  \\
   h_2' & = -\frac{h_2 \left(h_1 \left(h_2 v^2+\left(\mu ^2-1\right) \left(K \left(\mu
   ^2-1\right)+4\right)\right)+\mu ^2\right)}{\mu  \left(\mu ^2-1\right)} \ ,
   \label{eqno2}
\end{align}
where a prime denotes derivative with respect to $\mu$.
From \eqref{eqno1}, \eqref{eqno2}
we extract an ODE for the product $h_1 \, h_2$,
which is solved by
\beq \label{prodeq}
h_1 \, h_2 = \frac{\mu^2}{S + v^2 - S \, \mu^2} \ ,
\eeq
with $S$ an integration constant.
Using \eqref{prodeq} in \eqref{eqno2}, we get an ODE for $h_2$,
with solution
\begin{align}
h_2 &= 
\frac{\left(\mu ^2-1\right) S^2 \left(K \left(\mu ^2-1\right)+12\right)+4 S v^2 \left(K
   \left(\mu ^2-1\right)-6\right)-8 K v^4}{3 \left(\mu ^2-1\right) S^3}
   + B \, \frac{\sqrt{S + v^2 - S \, \mu^2}}{1-\mu^2} \ ,
\end{align}
where $B$ is an arbitrary constant.
It is convenient to introduce a new coordinate $t$
and parameters $a$, $b$ via
\beq
S + v^2 - S \, \mu^2 = v^2 \, t^2 \ , \qquad
S = - \frac{K}{3} \, a^2 \, v^2 \ , \qquad
B = \frac{b}{a^6 \, v^3 \, (K/3)^2} \ . 
\eeq
In parametrizing $S$ in terms of $a$
we have assumed $S \le 0$, which is necessary
in order to have the correct range for the variable $t$.
The metric on $M_4$ can the be written as
\begin{align} \label{metric_with_t}
\frac{K}{3} ds^2 (M_4) &= 
\frac{1 - t^2}{P} \, dt^2
+ \frac{P}{4\,a^4 \, v^2 \, (1 - t^2)} \, D  \widetilde{\psi}^2
+ \frac{1 - t^2}{4 \, a^2} \, ds^2(S^2_\varphi)
 \ ,  \quad \rm{(checked)}
\end{align}
where $P$ is the following polynomial in $t$,
\beq
P(t) =
t^4 + 2 \, (2 \, a^2 - 3) \, t^2 + b \, t + 4 \, a^2 - 3 
\ .      \quad \rm{(checked)}
\eeq
This polynomial can be cast in the form
\begin{align}
P(t) &= (t_+ - t ) \, (t - t_-) h(t), \\
 h(t) &= \bigg[
  - t^2 - (t_+ + t_-) \, t  + \frac{
 3 -  ( t_+^2 + t_+ \, t_- + t_-^2 )  }{1 - t_+ \, t_- } \bigg] \ ,
\end{align}
with the identifications
\beq
a^2 = \frac{
3 - 6 \, t_+ \, t_- + (t_+^2 + t_+ \, t_- + t_-^2) \, t_+ \, t_-
}{4 \, (1 - t_+ \, t_-)}  \ , \qquad
b = \frac{(t_+ + t_-) \, (  3 - t_+^2 \, t_-^2 - t_+^2 - t_-^2 )}{1 - t_+ \, t_-} \ .
\eeq 
From now on, we regard $(t_+, t_-, v)$ as free parameters
of the solution,
with $a$ and $b$ considered as dependent quantities. 
In order to have a well-behaved solution,
$t_+$, $t_-$ must be chosen in such a way that
\beq
-1 \le t_- < t_+ \le 1 \ , \qquad
a^2 \ge 0 \ , \qquad
P >0 \quad  \text{ for } \quad t\in (t_-, t_+) \ .
\eeq
We must also ensure the absence of conical
singularities as $t \rightarrow t_\pm$. The metric for the fiber $S^2$ in these regions is given as
\begin{align}
t \to t_\pm ,&  \quad  R^2 = \mp\left( t - t_\pm\right)  , \quad  \frac{K}{3} ds^2 \cong A_\pm^2 \left[ dR^2 + \frac{1}{Q_\pm^2} R^2 D\widetilde{\psi}^2 \right]  + \frac{1-t_\pm^2}{a^2} \,ds^2(S^2_\varphi).
\end{align}  The coefficients are given as
\begin{equation}
A_\pm^2 = \frac{4(1-t_\pm^2)}{(t_+ -t_-)h(t_\pm)}, \qquad Q_\pm = \frac{4 v a^2 (1-t_\pm^2)}{(t_+ -t_-)h(t_\pm)}.  
\end{equation} Let's assume denote the period of  $\widetilde{\psi}$ as $2\pi \ell $ for come constant $\ell$.  We wish to understand the possible values of $\ell$ up to conical defects at the poles.  Similarly, we must also impose a quantization condition for the degree of the $S^1_{\widetilde{\psi}}$ over the $S^1_\varphi$ sphere.  From these considerations, we impose the following quantization conditions
\begin{equation}
\frac{Q_\pm}{ \ell} = n_\pm \in \mathbb{Z}, \qquad \frac{1}{2\pi \ell} \int_{S^2_\varphi} d \left(D  \widetilde{\psi} \right) = \frac{2v}{\ell} = p \in \mathbb{Z} .
\end{equation} in these expressions, the circle coordinate $\psi = \frac{1}\ell \widetilde{\psi}$ has period $2\pi$ and deficit angle of $\frac{2\pi}{n_\pm}$ at the pole $t =t_\pm$.  In general the solution are labeled by the parameters $(t_\pm, v, \ell)$ which must fixed in terms of the quantized parameters $(n_\pm, p)$.  For any choice of these quantized parameters, one can look for a solution.

We are interested in cases where $M_4$ is smooth and admit no conical defects.  This implies that we must take $n_\pm =1$.  Moreover, we are also considering the case where the degree of the bundle is $p=2$.  This leads to the equations,
\begin{equation}
\ell =v , \qquad \frac{(t_+ -t_-) (t_\pm^2 + t_+ t_- -3)}{3 - 6 \, t_+ \, t_- + (t_+^2 + t_+ \, t_- + t_-^2) \, t_+ \, t_-} =1.  
\end{equation}  By taking the ratio of the $\pm$ equations we find that $t_+^2 =t_-^2$.  Since the ends of the intervals cannot be the same, we find that the solution must be
\begin{equation}
t_+ = -t_- = a^2 =1.
\end{equation}  This is the sphere solution.  Confusing!!

\begin{comment}
\begin{equation}
0< -t_- = t_0 = t_+ \leq 1,  \quad v^2 = 2t_0\frac{ t_0^2 +3}{3+6 t_0^2-t_0^4}, \quad a^2 = \frac{3+6t_0^2 -t_0^4}{4(1+t_0^2)}.
\end{equation} The metric of the space is then
\begin{equation}
\frac{K}3 ds^2(M_4) = \frac{1-t^2}{P} dt^2+ \frac{P}{4 a^4 (1-t^2)} D\psi^2 + \frac{1-t^2}{4 a^2} ds^2(S^2_\varphi) 
\end{equation} where $\psi$ have period $2\pi$.  The connection form and metric function can be written as
\begin{equation}
D\psi = d\psi + \cos(\theta) d\varphi, \qquad P(t) = (t_0^2 - t^2) \frac{4 - (1+t_0^2) (1+t^2)}{1+ t_0^2}.
\end{equation}  It is clear that $a^2$ is positive in the allowed range for $0<t_0\leq1$ and $P(t)$ is always non-negative.  
\end{comment}

\newpage
Near $t_+$ we can write
\beq
t_+ - t  = \xi \, R^2 \ ,
\eeq
with $\xi$ a positive constant, and $R$ a local radial coordinate.
In a small $R$ expansion,
\beq
P(t) = \xi \, R^2 \, Q_+  + \dots\ ,
\eeq
where
\beq
Q_+ = \frac{(t_+ - t_-) \, (1 - t_+^2) \, (3 - t_-^2 - 2 \, t_+ \, t_-)  }{1 - t_+ \, t_-} \ .
\eeq
The line element for $R \rightarrow 0$ has the form
\begin{align}
ds^2 (M_4) &= \frac{3}{K} \, 
\frac{4 \, (1 - t_+^2) \, \xi }{v^4 \, Q_+}
\bigg[
dR^2 
+\frac{v^2 \, Q_+^2}{4 \, (1-t_+^2)^2 \, a^4} \, R^2 \, D  \psi^2
+ \frac{v^4 \, Q_+}{16 \, \xi \, a^2} \, ds^2(S^2_\varphi)
\bigg] \ ,
\end{align}
which leads us to  
\beq
v = \frac{2 \, (1-t_+^2) \, a^2}{Q_+} = 
\frac{
3 - 6 \, t_+ \, t_- + (t_+^2 + t_+ \, t_- + t_-^2) \, t_+ \, t_-
}{2 \, (t_+ - t_-) \, (3 - t_-^2 - 2 \, t_+ \, t_-)}
 \ .
\eeq
(The sign of $v$ could be reversed by reversing the sign of $\psi$.)

A similar analysis can be performed for $t \rightarrow t_-$.
We find, however, that for generic $t_+$, $t_-$ the problem
is overconstrained, and we cannot ensure the absence of
conical singularities at both endpoints.
In order to have a smooth solution we must therefore have
\beq
(t_- , t_+) = (- t_0 , t_0)  \ .
\eeq
The metric is given by \eqref{metric_with_t}
with all quantities determined by the
single parameter $t_0$,
according to
\beq
P(t) = \frac{
(t ^2- t_0^2) \Big[ (1 + t_0^2) \, t^2   + t_0^2 -3 \Big]
}{1 + t_0^2} \ ,  \qquad
a^2 = 
\frac{3 + 6 \, t_0^2 - t_0^4 }{  4 \, (1 + t_0^2)} \ , \qquad
v = \frac{3 + 6 \, t_0^2 - t_0^4}{  4 \, t_0 \, (3 + t_0^2) } \ .
\eeq
In particular, if we set $t_0 = 1$ we obtain
\beq
ds^2(M_4) = \frac 3K \bigg[
\frac{16}{1-t^2} \, dt^2 + 4 \, (1-t^2) \, D\psi^2 + \frac 14 \, (1 -t^2) \, ds^2(S_\varphi^2)\bigg] \ , \qquad v = \frac 12  \ .
\eeq

********************************************************

\newpage

The metric \eqref{M4_metric} satisfies the Einstein condition
$R_{mn} = K \, g_{mn}$ provided that the metric functions $h_1$, $h_2$
are such that 
\begin{align}
h_1' & = \frac{h_1 \left(h_1 \left(3
   h_2+\left(\mu ^2-1\right)
   \left(K \left(\mu
   ^2-1\right)+4\right)\right)
   +\mu ^2-2\right)}{\mu 
   \left(\mu ^2-1\right)} \ ,  \label{diffno1} \\
h_2' & =    
-\frac{h_2 \left(h_1
   \left(h_2+\left(\mu
   ^2-1\right) \left(K
   \left(\mu
   ^2-1\right)+4\right)\right)
   +\mu ^2\right)}{\mu 
   \left(\mu ^2-1\right)}  \ ,   \label{diffno2}  \\
h_2'' & =   \frac{h_2}{\mu^2 (1-\mu^2)} \bigg[
\mu ^4 \left(h_1 \left(-h_1
   h_2
   K+K+8\right)+2\right)
   \nn \\
   & +\mu
   ^2 \left(h_1 \left(h_2
   \left(2 h_1
   (K-2)+5\right)-2
   (K+2)\right)+1\right)
   \nn \\
   &-h_1
   \left(h_1 h_2-1\right)
   \left(h_2+K-4\right)
   \bigg] \ ,   \label{diffno3}
\end{align}
where a prime denotes derivative with respect to $\mu$.
From \eqref{diffno1}, \eqref{diffno2} we derive the following relation for the product
$h_1 h_2$,
\beq
\mu \, (\mu^2 -1) \, (h_1 \, h_2)'  + 2 \, h_1 \, h_2 - 2 \, (h_1 \, h_2)^2 = 0 \ ,
\eeq
which is solved by
\beq \label{product_sol}
h_1 \, h_2 = \frac{\mu^2}{S+1 - S \, \mu^2} \ ,
\eeq
where $S$ is an arbitrary constant.
This quantity must be non-negative,
which requires $S+1 - S \, \mu^2 >0$.
The possible cases are
\begin{align}
-1 < \, &S  \le 0  \ , &  &\mu \in \mathbb R \ , \nn \\
&S > 0 \ ,  & &|\mu| < \sqrt{\frac{S+1}{S}} \ , \nn \\
&S \le -1   \ , & &|\mu|  > \sqrt{\frac{S+1}{S}} \ .
\end{align}
In the last case the range of $\mu$ is not acceptable.

Using \eqref{product}, equation \eqref{diffno2}
becomes
\begin{align}
\left(\mu ^2-1\right) \left(\left( S+1 -S \,  \mu ^2 \right)
 h_2'+\mu  \left(K \left(\mu
   ^2-1\right)+4\right)\right)+\mu 
   \left( S+2 - S \, \mu^2 \right) h_2= 0 \ ,
\end{align}
which is solved by
\begin{align}
h_2 = \frac{3 b S^3 \sqrt{ S+1 - S \, \mu^2}+\left(\mu
   ^2-1\right) S^2 \left(K \left(\mu
   ^2-1\right)+12\right)+4 S \left(K \left(\mu
   ^2-1\right)-6\right)-8 K}{3 \left(\mu ^2-1\right) S^3} \ ,
\end{align}
where $b$ in an arbitrary constant.
Notice that the argument of the square root
is the same quantity that enters $h_1 h_2$ in \eqref{product_sol},
and therefore the square root exists as soon as $h_1 \, h_2 \ge 0$.
Having determined $h_2$, $h_1$ is extracted from
\eqref{product_sol}, and the differential relation 
\eqref{diffno3} is automatically satisfied.

Let us define a new coordinate $t$ by
\beq
S+1 - S \, \mu^2 = t^2 \ .
\eeq
Since $\sqrt{t^2}$ enters $h_2$ accompanied by the
arbitrary constant $b$, we can choose the
square root branch $\sqrt{t^2} = t$ without loss
of generality.
We thus arrive at
\begin{align}
h_1 & =    -\frac{3 S \left(t^2-1\right)
   \left(S-t^2+1\right)}{t^2 \left(3 b S^3 t+K
   \left(t^4-6 t^2-3\right)-12 S
   \left(t^2+1\right)\right)}
    \ , \nn \\
    h_2 & = \frac{-3 \,  b \,  S^3 \,  t+K
   \left(-t^4+6 t^2+3\right)+12 S \left(t^2+1\right)}{3
   S^2 \left(t^2-1\right)} \ .
\end{align}
In terms of $t$, the metric  \eqref{M4_metric}  on $M_4$ reads
\begin{align}
ds^2(M_4) &= \frac{t^2}{S (S+1 -t^2)}   \, h_1 \,  dt^2 + \frac{1}{4} \,  h_2 \, D\psi^2 + \frac{t^2 -1}{4 \,S} ds^2(S^2_\varphi) \\
&= \frac{1}{S^2 h_2 }   dt^2 + \frac{1}{4} \,  h_2 \, D\psi^2 + \frac{t^2 -1}{4 \,S} ds^2(S^2_\varphi) .
\end{align}

When $S$ is negative, we define $a^2 = -\frac{3S}{K} $.  The metric and the function $h_2$ become
\begin{align}
\frac{K}{3} ds^2 (M_4) &= \frac{1}{ h} dt^2 + \frac{1}{4 a^4 } \,  h \, D\psi^2 + \frac{1}{4a^2} (1 -t^2) ds^2(S^2_\varphi) \\
h &= \frac{1}{1 -t^2} \left[ t^4 - (6-4a^2)t^2 + b t -3+4a^2  \right]
\end{align} where we have redefine $b$.  The coordinate $t$ is taken in the interval $[t_+,t_-]$ where $h_2$ vanish at the bounds.  In terms of these parameters, we can write 
\begin{align}
h &= (t_+ -t)(t-t_-) \tilde{h} (t), \\
\tilde{h}(t) &= \frac{1}{(1-t^2)}\left( \frac{3-(t_+ + t_-)^2 + t_+ t_-}{ 1-t_+ t_-} - (t_+ + t_-) t -t^2\right).
\end{align} The function $h(t)$ is required to be positive in the interval.  We can write $(a^2,b)$ in terms of the roots as
\begin{equation}
a^2 = \frac{3 - t_+ t_-[6- (t_+ + t_-)^2 +t_+ t_- ]}{4(1-t_+ t_-)}, \qquad b= \frac{(t_+ + t_-)(3-t_+^2 -t_-^2 -t_+^2 t_-^2)}{1-t_+ t_-}.  
\end{equation} In addition to the positivity of $h(t)$, the parameters $t_\pm$ are constrained by the condition
\begin{equation}
t_+ \leq 1, \quad t_->-1, \quad a^2\geq 0.  
\end{equation}
